# Supplementary material for: Maximizing and Satisficing in Multi-armed Bandits with Graph Information
Source: arXiv:2108.01152 source file (2022-11-20)
Supplement: Supplementary file 1 [file sampling_policies.tex]

\section{Better sampling strategies}\label{sec:better_sampling_policies}

Theorem~\ref{thm: sample_complexity} established a baseline w.r.t. sampling protocol by solving $T_{\text{sufficient}}$ for naive cyclic sampling policy (a sampling policy which doesn't exploit the graph properties). Note that, even if the sampling policy doesn't utilize any graph properties, the similarity graph is still being utilized in computing the mean estimate and the confidence widths. For the safe elimination of suboptimal arms, the ultimate goal of \algoname{} is to shrink the confidence bounds $\beta_i\sqrt{(t_{\text{eff}, i})^{-1}}$ as quickly as possible. Accordingly, a few intelligent sampling policies that exploit the graph structure of the problem is given as follows:
\begin{itemize}
    \item {\bf Marginal variance minimization (MVM):} Since picking any arm impacts the confidence widths of all arms in it's connected component, we pick the arm with the maximum variance. Specifically, $l = \underset{i\in A}{\arg\min}~ t_{\text{eff}, i} = \underset{i\in A}{\arg\max} ~[V_{T}^{-1}]_{ii}$, where $A$ is the set of indices of the arms under consideration. \\
    \item {\bf Joint variance minimization -- nuclear (JVM-N): }This variant is inspired from the concept of V-optimality~\cite{pmlr-v22-ji12}. This policy aims to select the arm that minimizes $\ell_2$ regression loss of the estimated vector $\hat{\pmb{\mu}}$, i.e. the confidence interval across all remaining arms in $A$. Specifically, $l = \underset{i\in A}{\arg\min} \|(V_{T} + \mathbf{e}_i\mathbf{e}_i^T)^{-1}\|_{*}$\\
    \item {\bf Joint variance minimization -- operator (JVM-O). }Taking inspiration from $\Sigma$-optimality~\cite{10.5555/3020847.3020904, ma2013sigma} the next policy can be stated as,
% \begin{align*}
  $l = \underset{i\in A}{\arg\min} \|(V_{T} + \mathbf{e}_i\mathbf{e}_i^T)^{-1}\|_{\text{op}}   = 
      \underset{i\in A}{\arg\max} \frac{\|\text{Row}_i(V_{T}^{-1})\|^2_2}{1+ [(V_T^{-1})_{ii}]}$
% \end{align*}
\end{itemize}
% Any additional derivation required for the above policies is provided in Appendix~\ref{app:sampling_policies}. 

% \section{Sampling policies}\label{app:sampling_policies}

The main objective of sampling policies is to   \textit{decrease} the value of $[V_{T}^{-1}]_{ii}$ for every arm $i$ as fast as possible. The notion of \textit{decrease} leads to different sampling policies for \algoname{}. The algorithm chooses the arm which maximizes this notion of decreases. 

The objective of the sampling policy \textbf{Joint variance minimization -- operator (JVM-O)} is equivalent to: 
\begin{align}
    % &\ \max_{k\in A} \|V_{T}^{-1}\|_{op} - \|\left(V_{T} + \mathbf{e}_k\mathbf{e}_k^T\right)^{-1}\|_{op}\nonumber\\
    \max_{k\in A} \sum_{j\in [n]}|(V_T^{-1})_{k, j}| -|\left(V_{T} + \mathbf{e}_k\mathbf{e}_k^T\right)^{-1}_{k,j}|
    % =  \max_{k\in A} \sum_{j\in [n]}\left(|\langle \mathbf{e}_{k}V_{T}^{-1}\mathbf{e}_{j}\rangle| -|\langle \mathbf{e}_{k}\left(V_{T} + \mathbf{e}_k\mathbf{e}_k^T\right)^{-1}\mathbf{e}_{j}\rangle|\right)\nonumber
\end{align}

Using Sherman-morrison rank 1 update we split the summation into different cases: 
\begin{itemize}
    \item For $j=k$,
\begin{align}
    &\ |\langle \mathbf{e}_{k}V_{T}^{-1}\mathbf{e}_{k}\rangle| -|\langle \mathbf{e}_{k}\left(V_{T} + \mathbf{e}_k\mathbf{e}_k^T\right)^{-1}\mathbf{e}_{k}\rangle|   =  \frac{\|\mathbf{e}_k\|^4_{V_T^{-1}}}{1+\|\mathbf{e}_k\|^2_{V_T^{-1}}}
\end{align}
\item For all connected-nodes of $j\in \mathcal{N}_k$,
\begin{align}
    &\ |\langle \mathbf{e}_{k}V_{T}^{-1}\mathbf{e}_{j}\rangle| -|\langle \mathbf{e}_{k}\left(V_{T} + \mathbf{e}_k\mathbf{e}_k^T\right)^{-1}\mathbf{e}_{j}\rangle|  =  \frac{\langle \mathbf{e}_j, \mathbf{e}_k\rangle^2_{V_T^{-1}}}{1+ \|\mathbf{e}_k\|^2_{V_T^{-1}}}
\end{align}
\item For all other non-connected $j\notin \mathcal{N}_k, i\neq k$,
\begin{align}
    |\langle \mathbf{e}_{k}V_{T}^{-1}\mathbf{e}_{i}\rangle| -|\langle \mathbf{e}_{k}\left(V_{T} + \mathbf{e}_k\mathbf{e}_k^T\right)^{-1}\mathbf{e}_{i}\rangle| =  0
\end{align}
\end{itemize}
Hence the sampling policy decides on the arm to sample based on the following optimization problem, 
\begin{align}
     \sum_{j\in [n]}|(V_T^{-1})_{k, j}| -|\left(V_{T} + \mathbf{e}_k\mathbf{e}_k^T\right)^{-1}_{k,j}|  &\ = \frac{\|\mathbf{e}_k\|^4_{V_T^{-1}}+\sum_{j\in \mathcal{N}_k}\langle\mathbf{e}_i, \mathbf{e}_k\rangle^2_{V_T^{-1}}}{1+ \|\mathbf{e}_k\|^2_{V_T^{-1}}}\nonumber\\ 
    % = &\ \max_{e_k\in A}\frac{\langle\mathbf{e}_k, \mathbf{e}_k\rangle^2_{V_T^{-1}}+\sum_{j\in \mathcal{N}_k}\langle\mathbf{e}_i, \mathbf{e}_k\rangle^2_{V_T^{-1}}}{1+ \|\mathbf{e}_k\|^2_{V_T^{-1}}}\nonumber\\
    % = &\ \max_{e_k\in A}\frac{[(V_T^{-1})_{kk}]^2+\sum_{j\in \mathcal{N}_k}[(V_T^{-1})_{kj}]^2}{1+ \|\mathbf{e}_k\|^2_{V_T^{-1}}}\nonumber\\
    % = &\ \max_{k\in A}\frac{[(V_t^{-1})_{kk}]^2+\sum_{j\in \mathcal{N}_k}[(V_T^{-1})_{kj}]^2}{1+ [(V_T^{-1})_{kk}]}\nonumber\\
    &\ = \frac{\|\text{Row}_k(V_{T}^{-1})\|^2_2}{1+ [(V_T^{-1})_{kk}]}\nonumber
\end{align}

Hence we try to find the arm $k$ within the remaining arms in consideration which maximizes $\frac{\|\text{Row}_k(V_{T}^{-1})\|^2_2}{1+ [(V_T^{-1})_{kk}]}$.
